# Supplementary material for: Lattice dynamics and polarization-dependent phonon damping in $\alpha$-phase FeSi$_{2}$ nanoislands
Source: arXiv:2003.02969 ancillary file (2020-03-06)
Supplement: Supplementary file 1 [file SM.pdf]

# Lattice dynamics and polarization-dependent phonon damping in $\alpha$-phase $FeSi_2$ nanoislands

# Supplemental Material

J. Kalt[1,2], M. Sternik[3], B. Krause[2], I. Sergueev[4], M. Mikolasek[5], D. Bessas[5], O. Sikora[3], T. Vitova[6], J. Göttlicher[2], R. Steininger[2], P. T. Jochym[3], A. Ptok[3], O. Leupold[4], H.-C. Wille[4], A. I. Chumakov[5], P. Piekarz[3], K. Parlinski[3], T. Baumbach[1,2] and S. Stankov[1,2]

[1]Laboratory for Applications of Synchrotron Radiation, Karlsruhe Institute of Technology, *D-76131* Karlsruhe, Germany

[2]Institute for Photon Science and Synchrotron Radiation, Karlsruhe Institute of Technology, *D-76344* Eggenstein-Leopoldshafen, Germany

[3]Institute of Nuclear Physics, Polish Academy of Sciences, *PL-31342* Kraków, Poland

[4]Deutsches Elektronen-Synchrotron, *D-22607* Hamburg, Germany

[5]ESRF - The European Synchrotron, *F-38000* Grenoble, France

[6]Institute for Nuclear Waste Disposal, Karlsruhe Institute of Technology, *D-76344* Eggenstein-Leopoldshafen, Germany

## 1 Calculation of the direction-projected phonon density of states

The phonon normal modes are obtained by solving the eigenvalue problem of the dynamical matrix $D(\boldsymbol{k})$:

$$D(\boldsymbol{k})\boldsymbol{e}(\boldsymbol{k},j) = \omega^2(\boldsymbol{k},j)\boldsymbol{e}(\boldsymbol{k},j) \tag{1}$$

where $\omega(\boldsymbol{k},j)$ denote the phonon frequencies for wave vector $\boldsymbol{k}$ and phonon dispersion band index $j$, and $\boldsymbol{e}(\boldsymbol{k},j)$ are the polarization vectors. The frequency distribution of the normal modes is described by the phonon density of states (PDOS) g($\omega$), defined as:

$$g(\omega) = \frac{1}{N}\sum_j \int\limits_{BZ} \delta(\omega - \omega(\boldsymbol{k},j))d^3\boldsymbol{k} \tag{2}$$

where $N$ is the number of states and BZ stands for Brillouin zone.

Generally, we can define the symmetric tensor $G^{\mu}_{il}(\omega)$:

$$G^{\mu}_{il}(\omega) = \frac{1}{N}\sum_{j}\int\limits_{BZ} e^{\mu}_{i}(\boldsymbol{k},j)[e^{\mu}_{l}(\boldsymbol{k},j)]^{*}\delta(\omega-\omega(\boldsymbol{k},j))d^{3}\boldsymbol{k} \tag{3}$$

where $\mu$ denotes an individual atom and the indexes $i$, $l$ define the Cartesian components of the polarization vector. The diagonal elements, $G^{\mu}_{xx}(\omega)$, $G^{\mu}_{yy}(\omega)$, and $G^{\mu}_{zz}(\omega)$, describe the PDOS projected along the $x$, $y$ and $z$ axis, respectively. The PDOS projected along an arbitrary direction $\boldsymbol{\kappa}$ can be calculated from $G^{\mu}_{il}(\omega)$ by:

$$g^{\mu}_{\boldsymbol{\kappa}}(\omega) = \sum_{i,l=1}^{3}\kappa_i\kappa_l G^{\mu}_{il}(\omega) \tag{4}$$

where $\kappa_i$ are the Cartesian components of $\boldsymbol{\kappa}$.

The PDOS measured by nuclear inelastic scattering (NIS) can be directly calculated from Eq. (4) assuming that $\boldsymbol{\kappa}$ is oriented along the wave vector of the incident X-ray beam, and $\mu$ denotes the Mössbauer-active isotope.

As discussed in the paper, three different domain orientations of $\alpha$-phase $FeSi_2$ are present on the Si(111) surface. When the X-ray beam is oriented along Si$\langle\bar{1}10\rangle$, three crystallographic directions of the $\alpha$-$FeSi_2$ domains are parallel to the wave vector of the incident photons, namely $[\bar{1}10]$, $[\bar{2}01]$ and $[0\bar{2}1]$. The components of these vectors have to be expressed in Cartesian coordinates using the lattice constants $a = 2.727$ Å and $c = 5.14$ Å (here we use the tensile strained $\alpha$-$FeSi_2$ unit cell with lattice parameters increased by 1%) and normalized:

$$\boldsymbol{\kappa}_{[\bar{1}10]} = \frac{1}{\sqrt{2}}[-1,1,0]; \tag{5}$$

$$\boldsymbol{\kappa}_{[\bar{2}01]} = \frac{1}{\sqrt{4a^2+c^2}}[-2a,0,c]; \tag{6}$$

$$\boldsymbol{\kappa}_{[0\bar{2}1]} = \frac{1}{\sqrt{4a^2+c^2}}[0,-2a,c]. \tag{7}$$

The PDOS calculated for the above vectors using Eq. (4) are shown in Fig. 1 [left panels (a)-(c), dashed lines]. In the PDOS spectrum of the first domain [Fig. 1(a)] the peak originating from the $z$-polarized phonons (around 20 meV) is absent, as the $z$ axis is perpendicular to the wave vector of the

incident photons. Due to symmetry with respect to the direction of the photon wave vector, the crystallographic vectors $[\bar{2}01]$ and $[0\bar{2}1]$ lead to equal contributions.

Assuming that these three domains are formed with the same probability, we obtain the theoretical PDOS, $g_{sum}(\omega)$:

$$g_{sum}(\omega) = \frac{1}{3}\left(g_{[\bar{1}10]}(\omega) + g_{[\bar{2}01]}(\omega) + g_{[0\bar{2}1]}(\omega)\right) \tag{8}$$

The calculated $g_{sum}(\omega)$ reproduces precisely the peak positions of the spectrum measured for S2 along Si$\langle\bar{1}10\rangle$ as it is shown in Fig. 1(d). The agreement between calculated and measured peak intensities is also sufficiently good.

In the same way the calculations were done for the $\alpha$-$FeSi_2$ directions parallel to Si$\langle 11\bar{2}\rangle$ (i.e. $[\bar{1}\bar{1}1]$, $[2\bar{4}1]$ and $[4\bar{2}1]$), and the respective plots are shown in the right panels of Fig. 1. While we get different components of the PDOS for the respective directions, the $g_{sum}(\omega)$ plotted in Fig. 1(d) and (h) are very similar. Therefore, despite the vibrational anisotropy observed for $xy$- and $z$-polarized phonons of $\alpha$-$FeSi_2$, the superposition of spectra of the specific crystal directions measured in our experiment leads to the observed vibrational isotropy.

As a next step, we calculate the PDOS considering only the diagonal components of $G^{\mu}_{il}(\omega)$. For this purpose we can rewrite Eq. (4) in a form:

$$\begin{aligned} g_{sum}(\omega) =& \frac{1}{3}\left((\kappa^x_{[\bar{1}10]})^2 + (\kappa^x_{[\bar{2}01]})^2 + (\kappa^x_{[0\bar{2}1]})^2\right) G_{xx}(\omega) \\ &+\frac{1}{3}\left((\kappa^y_{[\bar{1}10]})^2 + (\kappa^y_{[\bar{2}01]})^2 + (\kappa^y_{[0\bar{2}1]})^2\right) G_{yy}(\omega) \\ &+\frac{1}{3}\left((\kappa^z_{[\bar{1}10]})^2 + (\kappa^z_{[\bar{2}01]})^2 + (\kappa^z_{[0\bar{2}1]})^2\right) G_{zz}(\omega) \end{aligned} \tag{9}$$

Due to the tetragonal symmetry of the crystal $G_{xx} = G_{yy}$. The values of the coefficients before $G_{xx}$, $G_{yy}$ and $G_{zz}$ are 0.3428, 0.3428 and 0.3144, respectively, for Si$\langle\bar{1}10\rangle$. The same procedure used for Si$\langle 11\bar{2}\rangle$ leads to similar prefactors (0.3432, 0.3432 and 0.3136).

The calculated spectra are shown in Fig. 1 (solid lines) and cannot be distinguished from the data considering additionally the off-diagonal tensor elements (dashed lines). The off-diagonal tensor elements are much smaller and partially cancel out, therefore their influence on $g_{sum}$ is negligible.

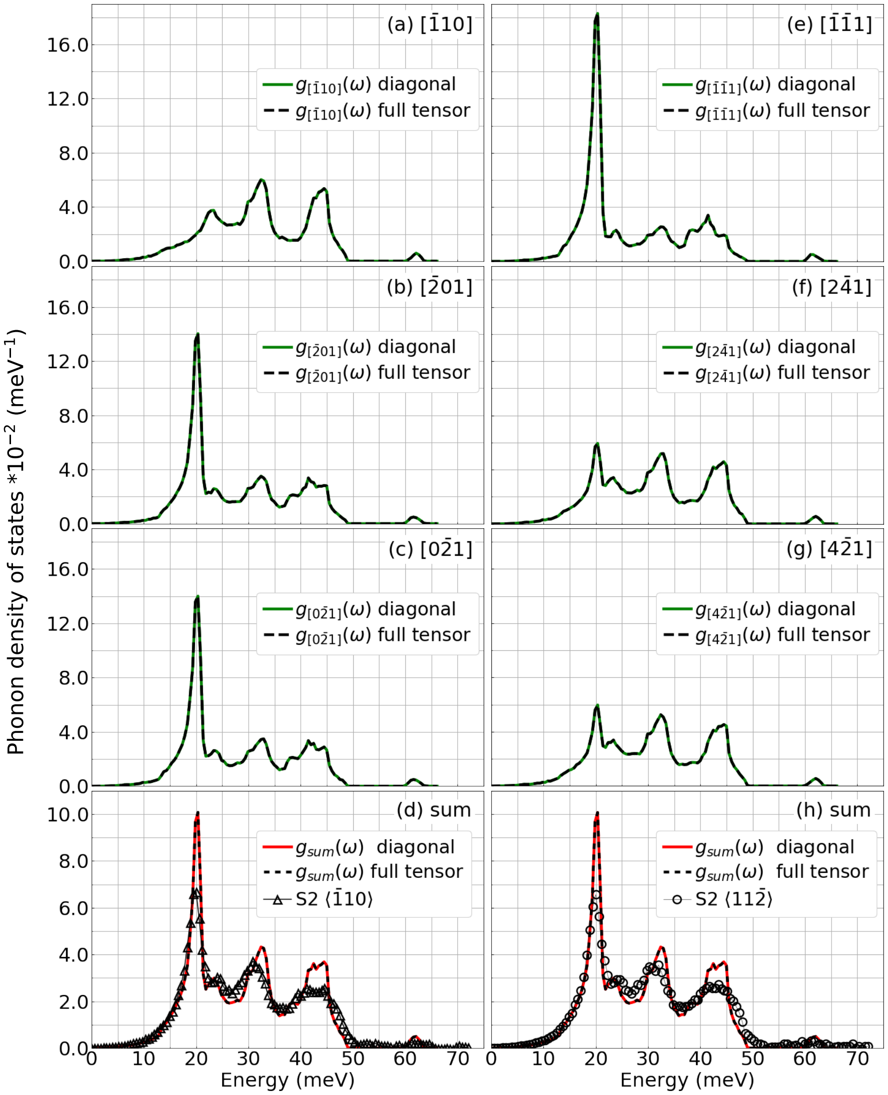


Figure 1: *Ab initio* calculated Fe-partial PDOS of $\alpha$-FeSi$_2$ projected along the indicated crystal directions. Panels from (a) to (c) show the spectra of the $\alpha$-FeSi$_2$ crystal directions parallel to Si$\langle\bar{1}10\rangle$, while from (e) to (g) the $\alpha$-FeSi$_2$ crystal directions parallel to Si$\langle 11\bar{2}\rangle$ are depicted, according to the epitaxial relationship described in the paper. In (d) and (h) the respective normalized sum, assuming a 1/3 contribution of each projection, is depicted and compared to the experimental results for S2. In each graph the results obtained under consideration of all tensor elements (dashed black line) are compared to the results derived by only considering the diagonal elements of the tensor (solid green/red line).

## 2 Additional fit results

As described in the paper, the experimental PDOS was modeled by the function $g_{th}(E, Q_{xy}, Q_z)$ defined as:

$$g_{th}(E, Q_{xy}, Q_z) = A_{xy}\, g_{xy}(E, Q_{xy}) + A_z\, g_z(E, Q_z) \tag{10}$$

where $g_{xy}$ and $g_z$ are the *ab initio* calculated Fe-partial PDOS ($G_{xx} = G_{yy}$ and $G_{zz}$, respectively), convoluted with the damped harmonic oscillator (DHO) function. The coefficients $A_{xy}$ and $A_z$:

$$A_{xy} = \frac{1}{3}\left((\kappa^{x}_{[\bar{1}10]})^2 + (\kappa^{x}_{[\bar{2}01]})^2 + (\kappa^{x}_{[0\bar{2}1]})^2\right) + \frac{1}{3}\left((\kappa^{y}_{[\bar{1}10]})^2 + (\kappa^{y}_{[\bar{2}01]})^2 + (\kappa^{y}_{[0\bar{2}1]})^2\right),$$
$$A_z = \frac{1}{3}\left((\kappa^{z}_{[\bar{1}10]})^2 + (\kappa^{z}_{[\bar{2}01]})^2 + (\kappa^{z}_{[0\bar{2}1]})^2\right)$$

are the contributions of the normalized components of the crystallographic vectors to the experimental PDOS measured along Si$\langle\bar{1}10\rangle$.

Using Eq. (10), the experimental spectra obtained along Si$\langle\bar{1}10\rangle$ (Fig. 2) and Si$\langle 11\bar{2}\rangle$ (Fig. 3) were fitted with two different approaches. In the first approach, we assumed $Q_{xy} = Q_z$, i.e. with the $xy$ and $z$ contributions experiencing the same damping [Fig. 2(a)-(f) and Fig. 3 (a)-(e)]. In the second approach, $Q_{xy}$ and $Q_z$ were independent parameters [Fig. 2(g)-(l) and Fig. 3(f)-(j)]. In all fits $A_{xy}$ and $A_z$ were fixed to the theoretically predicted values of 0.69 and 0.31, respectively. For S1-S3 both approaches lead to very similar results, whereas for S4-S6 the damping of the peaks of the $xy$-polarized phonons at 33 meV and 45 meV is overestimated if one common $Q$ is used. In the left panels, the ratio between the sum of squared residuals obtained by fitting with one common $Q$ ($rss^2_Q$) and the sum of squared residuals of the respective sample obtained from the fit conducted with independent $Q_{xy}$ and $Q_z$ ($rss^2_{Q_{xy}Q_z}$) are given. For S1 and S2 the values are the same for both approaches, for S3 the sum of squared residuals is increased by 10% if one common $Q$ is assumed. For S4-S6 the ratio increases sharply. For the spectra measured along Si$\langle 11\bar{2}\rangle$ this effect is also present.

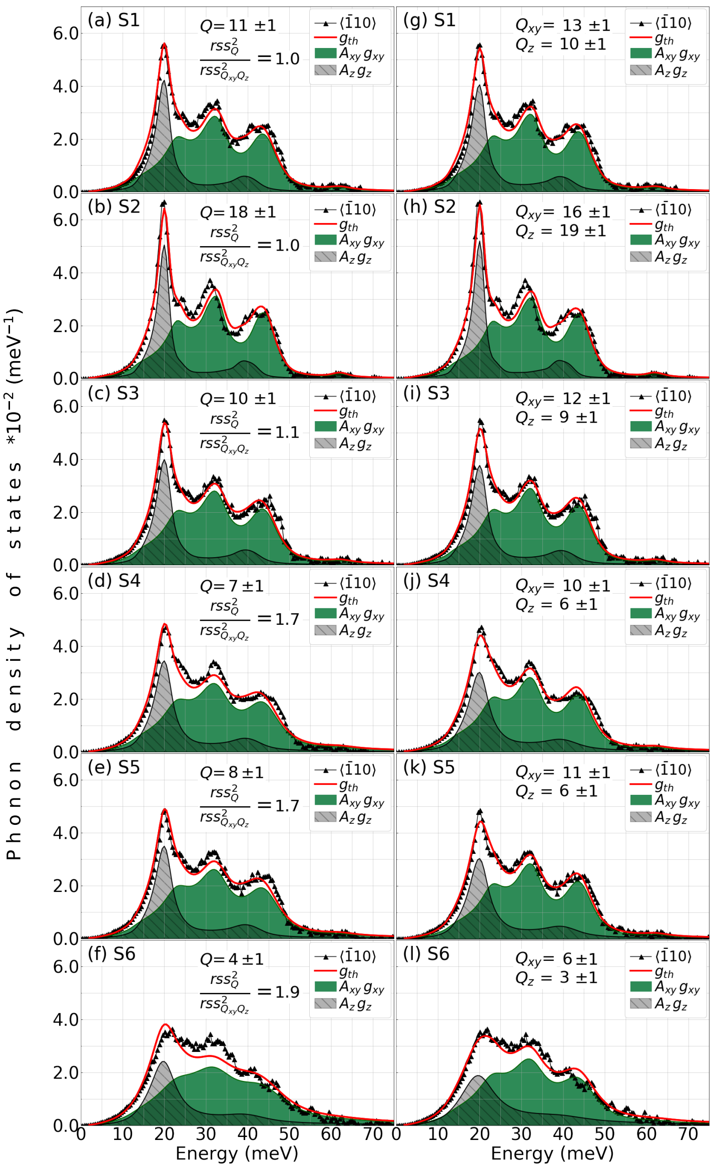


Figure 2: Fe-partial PDOS of the indicated samples measured along Si$\langle\bar{1}10\rangle$. The experimental data is compared with the respective result for $g_{th}$, which is decomposed to its weighted $xy$ ($A_{xy}\, g_{xy}$) and $z$ ($A_z\, g_z$) contributions. The left column (a)-(f) shows the fit results obtained under the assumption $Q_{xy} = Q_z$, in the right column (g)-(l) $Q_{xy}$ and $Q_z$ are independent parameters. In the left panels, the ratio between the sum of squared residuals obtained by fitting with one common $Q$ ($rss^2_Q$) and the sum of squared residuals of the respective sample obtained from the fit conducted with independent $Q_{xy}$ and $Q_z$ ($rss^2_{Q_{xy}Q_z}$) are given.

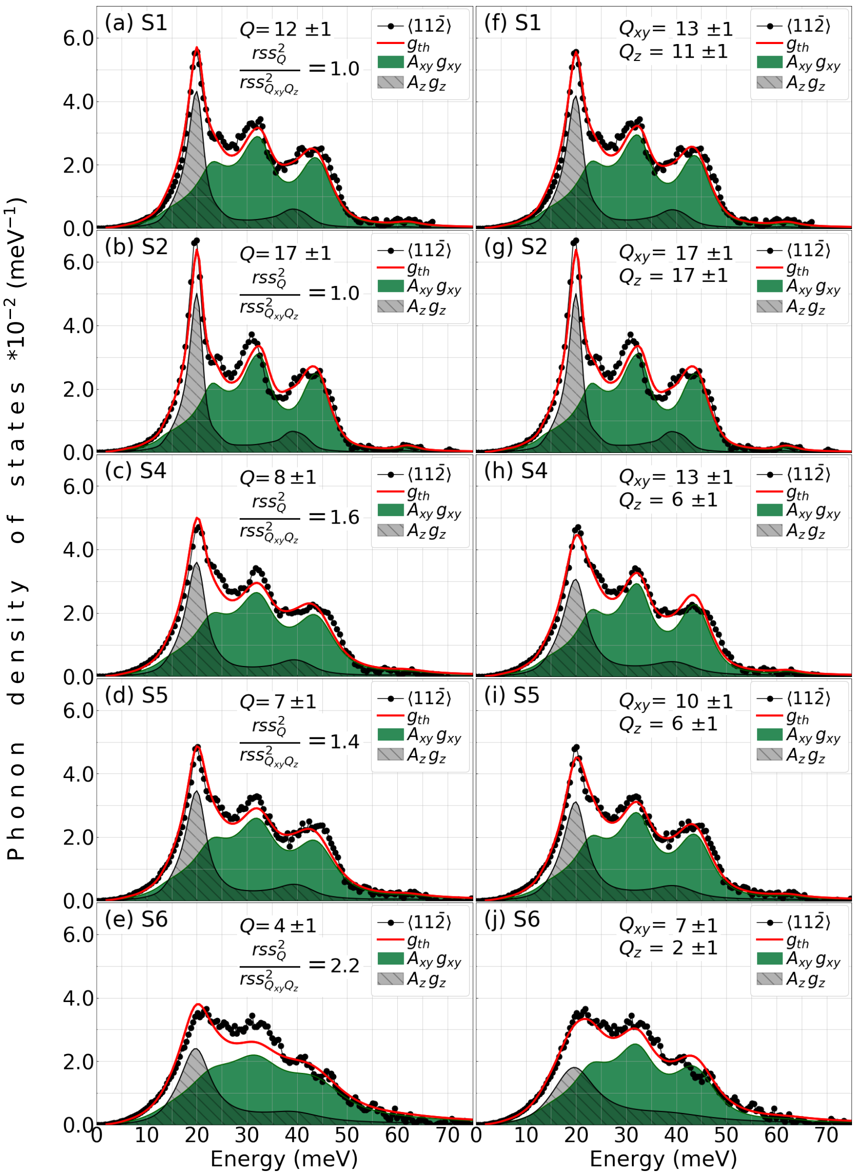


Figure 3: Fe-partial PDOS of the indicated samples measured along Si$\langle 11\bar{2} \rangle$. The experimental data is compared with the respective result for $g_{th}$, which is decomposed to its weighted $xy$ ($A_{xy}\, g_{xy}$) and $z$ ($A_z\, g_z$) contributions. The left column (a)-(e) shows the fit results obtained under the assumption $Q_{xy} = Q_z$, in the right column (f)-(j) $Q_{xy}$ and $Q_z$ are independent parameters. In the left panels, the ratio between the sum of squared residuals obtained by fitting with one common $Q$ ($rss_Q^2$) and the sum of squared residuals of the respective sample obtained from the fit conducted with independent $Q_{xy}$ and $Q_z$ ($rss^2_{Q_{xy}Q_z}$) are given.

# 3 Reduced PDOS

According to the Debye model, the low-energy part of the PDOS g(E) can be described by $g(E) = \alpha E^2$. The coefficient $\alpha$ can be used to quantify the enhancement of low-energy states in nanostructures. In Fig. 4 the reduced PDOS (g(E)/E$^2$) of S1-S6 is plotted. The insets show the $\alpha$ values obtained in the range from 4 - 10 meV as a function of average island height, normalized to the value of $\alpha_{S1}$.

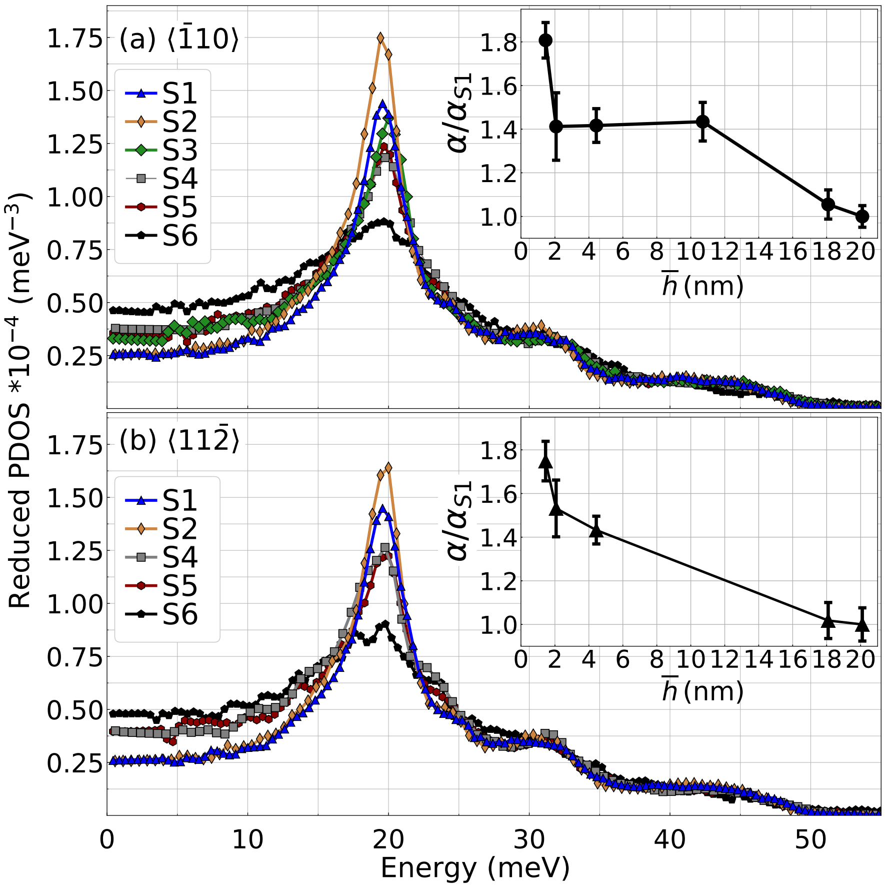


Figure 4: Fe-partial reduced PDOS (g(E)/E$^2$) of the indicated samples measured along Si$\langle\bar{1}10\rangle$ (a) and Si$\langle 11\bar{2}\rangle$ (b). The insets show the coefficient $\alpha$ as a function of average island height, normalized to the value of $\alpha_{S1}$.

## 4 XANES spectra and EXAFS Fourier transform

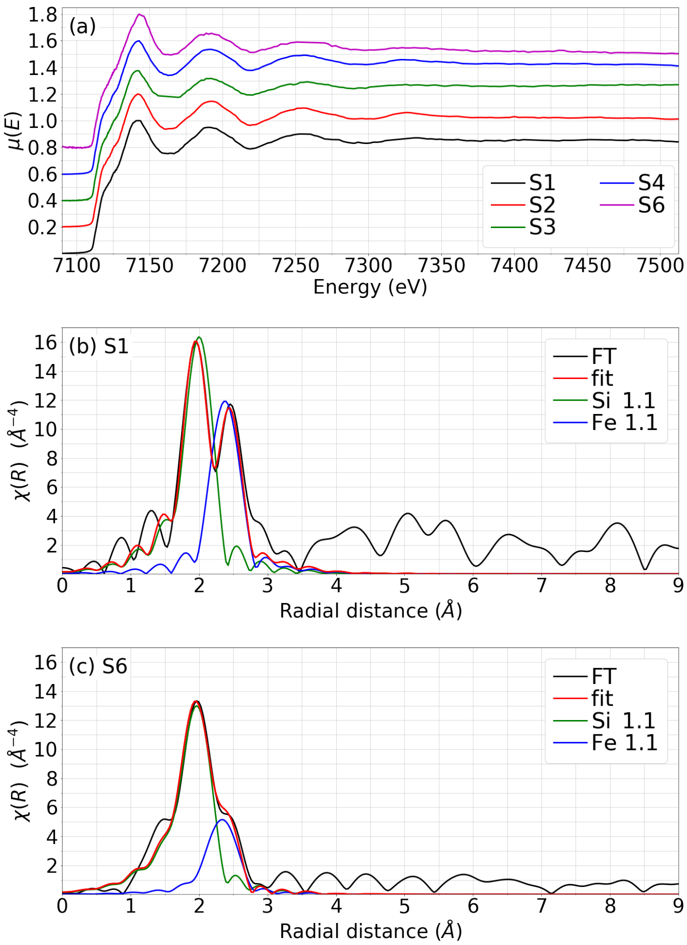


Figure 5: (a) Normalized Fe K-edge X-ray absorption near edges structure (XANES) spectra of the indicated samples. The spectra are shifted by 0.2 for clarity. (b) and (c) depict the Fourier transform of the EXAFS spectra shown in Fig. 5 in the main paper, together with the respective fits and element-resolved subspectra.
